# Supplementary material for: Device-Aware Routing and Scheduling in Multi-Hop Device-to-Device Networks
Source: arXiv:1708.06475 source file (2017-08-22)
Supplement: Supplementary file 1 [file appendixA.tex]

\section*{\label{sec:Th1_proof_unicast}Appendix A: Proof of Theorem~\ref{eec_theorem1} for Unicast Setup}
{\em Stability Region:}
Let $(A_{k})$ be the vector of arrival rates $\forall k \in \Nset$. The source-centric stability region $\Lambda_s$ is defined as the closure of all arrival rates that can be stably  transmitted in the network considering all possible routing and scheduling policies. The stably transmitted arrival rates $(A_{k})$ satisfy the following flow conservation constraints.
\begin{align}
\label{eq:appC_SC_stab_2_1}
& x_{k,k} + \sum_{n \in \Nset - \{k\}} x_{n,k} \geq A_{k}, \forall k \in \Nset  \\
\label{eq:appC_SC_stab_2_2}
& h_{n,k} \geq x_{n,k}, \forall k \in \Nset, n \in \Nset - \{k\}
\end{align} In other words, $\Lambda_{s} = \{(A_{k}) |$ Eq.~(\ref{eq:appC_SC_stab_2_1}), Eq.~(\ref{eq:appC_SC_stab_2_2}), $ x_{n,k} \geq 0, h_{n,k} \geq 0$, $\forall n, k \in \Nset \}$. Now, let us consider the stability region of the device-centric model.

Eqs.~(\ref{eq:appC_SC_stab_2_1}), (\ref{eq:appC_SC_stab_2_2}) are expressed as;
\begin{align}
\label{eq:appC_SC_stab_3_1}
& x_{k,k} + \sum_{n \in \Nset - \{k\}} x_{n,k} = A_{k} + \delta_{k}, \forall k \in \Nset  \\
\label{eq:appC_SC_stab_3_2}
& h_{n,k} = x_{n,k} + \delta_{n,k}, \forall k \in \Nset, n \in \Nset - \{k\}
\end{align} where $\delta_{k}$ and $\delta_{n,k}$ are small positive constants.
Considering that the device-centric algorithm sets; $g_{k,s}^{k} = x_{k,k}$, $g_{k,n}^{k}=h_{n,k}$, $g_{n,s}^{k} = x_{n,k}+\beta$, Eqs.~(\ref{eq:appC_SC_stab_3_1}), (\ref{eq:appC_SC_stab_3_1}) are expressed as;
\begin{align}
\label{eq:appC_DC_stab_1_1}
& g_{k,s}^{k} + \sum_{n \in \Nset - \{k\}} (g_{n,s}^{k} - \beta) = A_{k} + \delta_{k}, \forall k \in \Nset  \\
\label{eq:appC_DC_stab_1_2}
& g_{k,n}^{k} = g_{n,s}^{k} - \beta + \delta_{n,k}, \forall k \in \Nset, n \in \Nset - \{k\}
\end{align} which can be expressed as;
\begin{align}
\label{eq:appC_DC_stab_2_1}
& g_{k,s}^{k} + \sum_{n \in \Nset - \{k\}} g_{n,s}^{k} = A_{k} + \delta_{k} + (N-1)\beta, \forall k \in \Nset  \\
\label{eq:appC_DC_stab_2_2}
& g_{n,s}^{k} = g_{k,n}^{k} + \beta - \delta_{n,k}, \forall k \in \Nset, n \in \Nset - \{k\}
\end{align}
By changing variables, we have;

\begin{align}
\label{eq:appC_DC_stab_3_1}
& g_{k,s}^{k} + \sum_{n \in \Nset - \{k\}} g_{k,n}^{k} = A_{k} + \delta_{k} + \sum_{n \in \Nset - \{k\}} \delta_{n,k}, \nonumber \\
& \forall k \in \Nset
\end{align}
\begin{align}
\label{eq:appC_DC_stab_3_2}
& g_{k,n}^{k} = g_{n,s}^{k} - \beta + \delta_{n,k}, \forall k \in \Nset, n \in \Nset - \{k\}
\end{align}
If $\beta$ is selected as $\beta > \delta =  \max\{\delta_{n,k}\}_{\forall n \in \Nset, k \in \Nset - \{k\}}$, we have;
\begin{align}
\label{eq:appC_DC_stab_4_1}
& g_{k,s}^{k} + \sum_{n \in \Nset - \{k\}} g_{k,n}^{k} \geq A_{k}, \forall k \in \Nset  \\
\label{eq:appC_DC_stab_4_2}
& g_{n,s}^{k} \geq g_{k,n}^{k}, \forall k \in \Nset, n \in \Nset - \{k\}
\end{align}
The device-centric stability region $\Lambda_{d}$ is defined as; $\Lambda_{d} = \{ (A_{k}) | $ Eq.~(\ref{eq:appC_DC_stab_4_1}), Eq.~(\ref{eq:appC_DC_stab_4_1}), $g_{n,s}^{k} \geq 0, g_{k,n}^{k} \geq 0, \forall n, k \in \Nset \}$.
%Note that the vector of arrival rates that are stably transmitted by the source-centric algorithm, \ie $(A_{k})$, $\forall k \in \Nset$ are stably supported by the device centric algorithm. The only difference is that

Note that Theorem~\ref{eec_theorem1} states that if channel states are i.i.d. over time slots, and the arrival rates $E[y_{t}(t)] = A_k, \forall k \in \Nset$ are interior of the stability region of cellular and local area links, \ie $\Lambda_d$, then DcC stabilizes the network and the total average queue sizes, including both virtual and real queues, are bounded for both unicast and broadcast setups. Next, we prove this statement for the unicast setup.

%Eq.~(\ref{eq:appC_DC_stab_4_1}) and Eq.~(\ref{eq:appC_DC_stab_4_2}) characterize the stability region of the device-centric scheme. The stability region of the device-centric system is smaller than the source-centric system by $\beta$ which could be arbitrarily small. Next, we show that DcC achieves this stability region.

{\em Stability Proof:}
Let $\boldsymbol H(t) = \{ \boldsymbol{{\lambda}(t)}, \boldsymbol{{\eta}(t)}, \boldsymbol{Q(t)} \}$ where $\boldsymbol{{\lambda}(t)} = \{{\lambda}_{k}(t)\}_{\forall k \in \Nset}$, $\boldsymbol{{\eta}(t)} = \{{\eta}_{n,k}(t)\}_{\forall k \in \Nset, \forall n \in \Nset-\{k\}}$, and $\boldsymbol{Q(t)} = \{Q_{n,k}(t)\}_{\forall k \in \Nset, \forall n \in \Nset-\{k\}}$.

%Let
%\begin{align} \label{eq:appC_allQueues_1}
%\boldsymbol H(t) = \{ \boldsymbol{{\lambda}(t)}, \boldsymbol{{\eta}(t)}, \boldsymbol{Q(t)} \}
%\end{align} where
%\begin{align} \label{eq:appC_allQueues_2}
%& \boldsymbol{{\lambda}(t)} = \{{\lambda}_{k}(t)\}_{\forall k \in \Nset} \nonumber \\
%& \boldsymbol{{\eta}(t)} = \{{\eta}_{n,k}(t)\}_{\forall k \in \Nset, \forall n \in \Nset-\{k\}} \nonumber \\
%& \boldsymbol{Q(t)} = \{Q_{n,k}(t)\}_{\forall k \in \Nset, \forall n \in \Nset-\{k\}} \nonumber \\
%\end{align}

Let the Lyapunov function be;
\begin{align} \label{eq:appC_lyap}
& L(\boldsymbol H(t)) =  \sum_{k \in \Nset} ({\lambda}_{k}(t))^{2} + \sum_{k \in \Nset} \sum_{n \in \Nset - \{k\}} ({\eta}_{n,k}(t))^{2} + \nonumber \\
& \sum_{k \in \Nset} \sum_{n \in \Nset-\{k\}} (Q_{n,k}(t))^{2}
\end{align}
The Lyapunov drift is;
\begin{align} \label{eq:appC_lyap_drift_1}
\Delta(\boldsymbol H(t)) = E[L(\boldsymbol H(t+1)) - L(\boldsymbol H(t)) | \boldsymbol H(t)]
\end{align} which is expressed as;
\begin{align} \label{eq:appC_lyap_drift_2}
& \Delta(\boldsymbol H(t)) =  E[\sum_{k \in \Nset} ({\lambda}_{k}(t+1))^{2} - \sum_{k \in \Nset} ({\lambda}_{k}(t))^{2} +  \sum_{k \in \Nset} \nonumber \\
& \sum_{n \in \Nset-\{k\}}   ({\eta}_{n,k}(t+1))^{2} - \sum_{k \in \Nset} \sum_{n \in \Nset-\{k\}} ({\eta}_{n,k}(t))^{2} +   \nonumber 
\\
&  \sum_{k \in \Nset} \sum_{n \in \Nset-\{k\}} (Q_{n,k}(t+1))^{2} - \sum_{k \in \Nset} \sum_{n \in \Nset-\{k\}}   \nonumber \\
&  (Q_{n,k}(t))^{2} | \boldsymbol H(t)]
\end{align} Considering the fact that $(\max[Q-b,0]+A)^{2} \leq Q^{2} + A^{2} + b^{2} + 2Q(A-b)$, Eq.~(\ref{eq:appC_lyap_drift_2}) is expressed as;
\begin{align}
& \Delta(\boldsymbol H(t)) \leq  E\biggl[ \sum_{k \in \Nset} \biggl(  \Bigl({\lambda}_{k}(t)\Bigr)^{2} + \Bigl({y}_{k}(t)\Bigr)^{2} + \Bigl({g}_{k,s}^{k}(t) + \nonumber \\
& \sum_{n \in \Nset - \{k\}} {g}_{k,n}^{k}(t)\Bigr)^{2} + 2{\lambda}_{k}(t) \Bigl({y}_{k}(t) - {g}_{k,s}^{k}(t) -  \sum_{n \in \Nset - \{k\}} \nonumber \\
& {g}_{k,n}^{k}(t) \Bigr)  - \Bigl({\lambda}_{k}(t)\Bigr)^{2} \biggr)
+ \sum_{k \in \Nset} \sum_{n \in \Nset-\{k\}} \biggl(  \Bigl({\eta}_{n,k}(t)\Bigr)^{2} \nonumber
\end{align}
\begin{align} \label{eq:appC_lyap_drift_3}
& + \Bigl({g}_{k,n}^{k}(t)\Bigr)^{2} + \Bigl({g}_{n,s}^{k}(t) \Bigr)^{2} + 2{\eta}_{n,k}(t) \Bigl({g}_{k,n}^{k}(t) -  \nonumber \\
& {g}_{n,s}^{k}(t) \Bigr) - \Bigl({\eta}_{n,k}(t)\Bigr)^{2} \biggr)
+ \sum_{k \in \Nset} \sum_{n \in \Nset-\{k\}} \biggl(  \Bigl(Q_{n,k}(t)\Bigr)^{2}  \nonumber \\ 
& + \Bigl({x}_{n,k}(t)\Bigr)^{2} + \Bigl({h}_{n,k}(t) \Bigr)^{2} + 2Q_{n,k}(t) \Bigl({x}_{n,k}(t) -  \nonumber \\
& {h}_{n,k}(t) \Bigr) - \Bigl(Q_{n,k}(t)\Bigr)^{2} \biggr) | \boldsymbol H(t)\biggr]
\end{align}
There exists a finite positive constant $B$ satisfying;
\begin{align} \label{eq:appC_lyap_B}
& B \geq E\biggl[ \sum_{k \in \Nset} ({y}_{k}(t))^{2}  + \sum_{k \in \Nset}
\bigl(  {g}_{k,s}^{k}(t) + \sum_{n \in \Nset - \{k\}} {g}_{k,n}^{k}(t) \bigr)^{2}  \nonumber \\
& + \sum_{k \in \Nset} \sum_{n \in \Nset-\{k\}} \bigl( ({g}_{k,n}^{k}(t))^{2} + ({g}_{n,s}^{k}(t))^{2} \bigr)
+ \sum_{k \in \Nset} \sum_{n \in \Nset-\{k\}} \nonumber \\
& \bigl( ({x}_{n,k}(t))^{2}  + ({h}_{n,k}(t))^{2} \bigr) | \boldsymbol H(t) \biggr]
\end{align}
By taking into account Eq.~(\ref{eq:appC_lyap_B}), Eq.~(\ref{eq:appC_lyap_drift_3}) is expressed as;
\begin{align} \label{eq:appC_lyap_drift_4}
& \Delta(\boldsymbol H(t)) \leq B + 2E\biggl[ \sum_{k \in \Nset} {\lambda}_{k}(t) \Bigl( {y}_{k}(t) - {g}_{k,s}^{k}(t) - \nonumber \\
& \sum_{n \in \Nset - \{k\}} {g}_{k,n}^{k}(t)  \Bigr) + \sum_{k \in \Nset} \sum_{n \in \Nset - \{k\}} {\eta}_{n,k}(t) \Bigl({g}_{k,n}^{k}(t) - \nonumber \\
& {g}_{n,s}^{k}(t) \Bigr) +  \sum_{k \in \Nset} \sum_{n \in \Nset-\{k\}} Q_{n,k}(t) \Bigl( {x}_{n,k}(t) - {h}_{n,k}(t)  \Bigl) \nonumber \\
& | \boldsymbol H(t)\biggr]
\end{align}
Since our algorithm (DcC) sets ${x}_{n,k}(t) = {g}_{n,s}^{k}(t) - \beta$ and ${h}_{n,k}(t) = {g}_{k,n}^{k}(t)$, Eq.~(\ref{eq:appC_lyap_drift_4}) is expressed as;
\begin{align} \label{eq:appC_lyap_drift_5}
& \Delta(\boldsymbol H(t)) \leq B + 2E\biggl[ \sum_{k \in \Nset} {\lambda}_{k}(t) \Bigl( {y}_{k}(t) - {g}_{k,s}^{k}(t) - \nonumber \\
& \sum_{n \in \Nset - \{k\}} {g}_{k,n}^{k}(t)  \Bigr) + \sum_{k \in \Nset} \sum_{n \in \Nset - \{k\}} {\eta}_{n,k}(t) \Bigl({g}_{k,n}^{k}(t) - \nonumber  \\
& {g}_{n,s}^{k}(t) \Bigr) + \sum_{k \in \Nset} \sum_{n \in \Nset-\{k\}} Q_{n,k}(t) \Bigl( {g}_{n,s}^{k}(t) - \beta - \nonumber \\
& {g}_{k,n}^{k}(t)  \Bigl) | \boldsymbol H(t)\biggr]
\end{align}
By arranging the terms, we have;
\begin{align} \label{eq:appC_lyap_drift_6}
& \Delta(\boldsymbol H(t)) \leq B - 2E\biggl[ \sum_{k \in \Nset} {\lambda}_{k}(t) \Bigl( {g}_{k,s}^{k}(t) + \sum_{n \in \Nset - \{k\}}  \nonumber \\
& {g}_{k,n}^{k}(t)  - {y}_{k}(t) \Bigr) + \sum_{k \in \Nset} \sum_{n \in \Nset - \{k\}} \Bigl( {\eta}_{n,k}(t) - Q_{n,k}(t) \Bigr) \nonumber \\
& \Bigl( {g}_{n,s}^{k}(t) -  {g}_{k,n}^{k}(t) \Bigr) + \sum_{k \in \Nset} \sum_{n \in \Nset-\{k\}} Q_{n,k}(t) \beta
| \boldsymbol H(t)\biggr]
\end{align}

The minimization of the right hand side of the drift inequality in Eq.~(\ref{eq:appC_lyap_drift_6}) corresponds to the cellular link scheduler in Eq.~(\ref{eq:cellular_scheduling}) and the local area link scheduler for unicast in Eq.~(\ref{eq:local_area_scheduling_unicast}).

Since $E[y_{k}(t)] = A_{k}$ and $(A_{k})$ is inside the stability region $\Lambda_{d}$, there exists a randomized policy with solution; $\oset{*}{g}_{k,s}^{k}$, $\oset{*}{g}_{k,n}^{k}$ satisfying;
\begin{align}
\label{eq:appC_comp_w_randomized_1}
& - E \biggl[ \Bigl( \oset{*}{g}_{k,s}^{k}(t) + \sum_{n \in \Nset - \{k\}} \oset{*}{g}_{k,n}^{k}(t) - {y}_{k}(t)   \Bigr)  \biggr] \leq  - \delta
\end{align}
\begin{align} \label{eq:appC_comp_w_randomized_2}
& - E \biggl[\Bigl( \oset{*}{g}_{n,s}^{k}(t) - \oset{*}{g}_{k,n}^{k}(t)   \Bigr)  \biggr] \leq - \Bigl(  \beta - \delta \Bigr)
\end{align}
%\begin{align} \label{eq:appC_comp_w_randomized_2}
%& - E \biggl[ \Bigl( {\eta}_{n,k}(t) - Q_{n,k}(t) \Bigr) \Bigl( \oset{*}{g}_{n,s}^{k}(t) - \oset{*}{g}_{k,n}^{k}(t)   \Bigr) | \boldsymbol H(t) \biggr] \leq \nonumber \\
%& - \Bigl( {\eta}_{n,k}(t) - Q_{n,k}(t) \Bigr) \Bigl(  \beta - \delta \Bigr)
%\end{align}

Since our algorithm, DcC, minimizes the right hand side of the drift inequality in Eq.~(\ref{eq:appC_lyap_drift_6}), the solution of DcC, \ie ${g}_{k,s}^{k}$, ${g}_{k,n}^{k}$ satisfy $- E [ \lambda_{k}(t)$ $( {g}_{k,s}^{k}(t)$ $+$ $\sum_{n \in \Nset - \{k\}}$ ${g}_{k,n}^{k}(t)$ $-$ ${y}_{k}(t) )$ $|$ $\boldsymbol H(t) ]$ $\leq$ $-$ $E [ \lambda_{k}(t)$ $( \oset{*}{g}_{k,s}^{k}(t)$ $+$ $\sum_{n \in \Nset - \{k\}}$ $\oset{*}{g}_{k,n}^{k}(t)$ $-$ ${y}_{k}(t)   )$ $|$ $\boldsymbol H(t) ]$ $\leq$  $-$ ${\lambda}_{k}(t)$ $\delta $ and $-$ $E [ ( {\eta}_{n,k}(t)$ $-$ $Q_{n,k}(t) )$ $({g}_{n,s}^{k}(t)$ $-$ ${g}_{k,n}^{k}(t)   )$ $|$ $\boldsymbol H(t) ]$ $\leq$ $-$ $E [ ( {\eta}_{n,k}(t)$ $-$ $Q_{n,k}(t) )$ $( \oset{*}{g}_{n,s}^{k}(t)$ $-$ $\oset{*}{g}_{k,n}^{k}(t)   )$ $|$ $\boldsymbol H(t) ]$ $\leq$  $-$ $( {\eta}_{n,k}(t)$ $-$ $Q_{n,k}(t) )$ $(  \beta$ $-$ $\delta )$.
By taking into account these inequalities, the drift inequality in Eq.~(\ref{eq:appC_lyap_drift_6}) is bounded as;
\begin{align} \label{eq:appC_lyap_drift_7}
& \Delta(\boldsymbol H(t)) \leq B - 2 \sum_{k \in \Nset} {\lambda}_{k}(t) \delta -  2 \sum_{k \in \Nset} \sum_{n \in \Nset - \{k\}}  {\eta}_{n,k}(t)  \nonumber \\
& (\beta - \delta)  -  2 \sum_{k \in \Nset} \sum_{n \in \Nset - \{k\}} Q_{n,k}(t) \delta
\end{align}
The time average of the Lyapunov drift in Eq.~(\ref{eq:appC_lyap_drift_7}) is;
\begin{align} \label{eq:appC_lyap_timeAvg_1}
& \limsup_{t \rightarrow \infty} \frac{1}{t} \sum_{\tau = 0}^{t-1} \frac{\Delta(\boldsymbol H(t))}{2} \leq \limsup_{t \rightarrow \infty} \frac{1}{t} \sum_{\tau=0}^{t-1} \biggl( \frac{B}{2} - \sum_{k \in \Nset}  \nonumber \\
& {\lambda}_{k}(\tau)  \delta - \sum_{k \in \Nset} \sum_{n \in \Nset - \{k\}} {\eta}_{n,k}(\tau) (\beta - \delta) -  \sum_{k \in \Nset}  \sum_{n \in \Nset - \{k\}} \nonumber \\
&  Q_{n,k}(\tau) \delta \biggl)
\end{align} which leads to

\begin{align} \label{eq:appC_lyap_timeAvg_2}
& \limsup_{t \rightarrow \infty} \frac{1}{t} \sum_{\tau=0}^{t-1} \biggl( \sum_{k \in \Nset} {\lambda}_{k}(\tau)  \delta -  \sum_{k \in \Nset} \sum_{n \in \Nset - \{k\}}  {\eta}_{n,k}(\tau)  \nonumber \\
& (\beta - \delta) -  \sum_{k \in \Nset} \sum_{n \in \Nset - \{k\}} Q_{n,k}(\tau) \delta \biggl) \leq \frac{B}{2}
\end{align} Since $\beta > \delta$, Eq.~(\ref{eq:appC_lyap_timeAvg_2}) concludes that the time average of the sum of the queues are bounded. This concludes the proof.
