# Supplementary material for: Device-Aware Routing and Scheduling in Multi-Hop Device-to-Device Networks
Source: arXiv:1708.06475 source file (2017-08-22)
Supplement: Supplementary file 2 [file appendixB.tex]

\section*{Appendix B: Proof of Theorem~\ref{eec_theorem1} for Broadcast Setup}
{\em Stability Region:} Let $(A_{k})$ be the vector of arrival rates $\forall k \in \Nset$. The source centric stability region for the broadcast setup, $\tilde{\Lambda}_{s}$, is defined as the closure of all arrival rates that can be stably transmitted in the network considering all possible routing and scheduling policies. The stably transmitted arrival rates $(A_{k})$ satisfy the following flow conservation constraints.
\begin{align}
\label{eq:appC_stab_reg_broadcast_1_1}
& x_{k,k} + \sum_{n \in \Nset - \{k\}} x_{n,k} \geq A_{k}, \forall k \in \Nset
\end{align}
\begin{align}
\label{eq:appC_stab_reg_broadcast_1_2}
& h_{n,k} \geq x_{n,k}, \forall k \in \Nset, n \in \Nset - \{k\}
\end{align}
\begin{align}
\label{eq:appC_stab_reg_broadcast_1_3}
& h_{n,k} \leq \sum_{\Jset \in \Hset | k \in \Jset, n \notin \Jset} f_{n,\Jset}, \forall n \in \Nset, k \in \Nset - \{n\}
\end{align} In other words, $\tilde{\Lambda}_{s} = \{ (A_{k}) | $ Eq.~(\ref{eq:appC_stab_reg_broadcast_1_1}), Eq.~(\ref{eq:appC_stab_reg_broadcast_1_2}), Eq.~(\ref{eq:appC_stab_reg_broadcast_1_3}), $x_{n,k} \geq 0, h_{n,k} \geq 0, \forall n,k \in \Nset, f_{n,\Jset} \geq 0, \forall n \in \Nset, \Jset \in \Hset \}$. Now, let us consider the stability region of the device-centric model. Eqs.~(\ref{eq:appC_stab_reg_broadcast_1_1}), (\ref{eq:appC_stab_reg_broadcast_1_2}), (\ref{eq:appC_stab_reg_broadcast_1_3}) are expressed as;
\begin{align}
\label{eq:appC_stab_reg_broadcast_2_1}
& x_{k,k} + \sum_{n \in \Nset - \{k\}} x_{n,k} = A_{k} + \delta_{k}, \forall k \in \Nset  \\
\label{eq:appC_stab_reg_broadcast_2_2}
& h_{n,k} = x_{n,k} + \delta_{n,k}, \forall k \in \Nset, n \in \Nset - \{k\}  \\
\label{eq:appC_stab_reg_broadcast_2_3}
& h_{n,k} = \sum_{\Jset \in \Hset | k \in \Jset, n \notin \Jset} f_{n,\Jset}, \forall n \in \Nset, k \in \Nset - \{n\}
\end{align}
Considering the fact that $g_{k,s}^{k} = x_{k,k}$, $g_{k,n}^{k} = h_{n,k}$, $g_{n,s}^{k} = x_{n,k} + \beta$; we have;
\begin{align}
\label{eq:appC_stab_reg_broadcast_3_1}
& g_{k,s}^{k} + \sum_{n \in \Nset - \{k\}} (g_{n,s}^{k} - \beta) = A_{k} + \delta_{k}, \forall k \in \Nset  \\
\label{eq:appC_stab_reg_broadcast_3_2}
& g_{k,n}^{k} = g_{n,s}^{k} - \beta + \delta_{n,k}, \forall k \in \Nset, n \in \Nset - \{k\}  \\
\label{eq:appC_stab_reg_broadcast_3_3}
& g_{k,n}^{k} = \sum_{\Jset \in \Hset | k \in \Jset, n \notin \Jset} f_{n,\Jset}, \forall n \in \Nset, k \in \Nset - \{n\}
\end{align} By rearranging variables, we have;
\begin{align}
\label{eq:appC_stab_reg_broadcast_4_v1}
& g_{k,s}^{k} + \sum_{n \in \Nset - \{k\}} \sum_{\Jset | k \in \Jset, n \notin \Jset} f_{n,\Jset} = A_{k} + \delta_{k} +  \nonumber \\
& \sum_{n \in \Nset - \{k\}} \delta_{n,k}, \forall k \in \Nset  \\
\label{eq:appC_stab_reg_broadcast_4_v2}
& g_{n,s}^{k} = \sum_{\Jset \in \Hset | k \in Jset, n \notin \Jset} f_{n,\Jset} + \beta - \delta_{n,k}, \forall k \in \Nset, \nonumber \\
& n \in \Nset - \{k\}
\end{align}
If $\beta$ is selected as $\beta > \delta =  \max\{\delta_{n,k}\}_{\forall n \in \Nset, k \in \Nset - \{k\}}$, we have;

\begin{align}
\label{eq:appC_stab_reg_broadcast_5_v1}
& g_{k,s}^{k} + \sum_{n \in \Nset - \{k\}} \sum_{\Jset | k \in \Jset, n \notin \Jset} f_{n,\Jset} \geq A_{k}, \forall k \in \Nset \\
\label{eq:appC_stab_reg_broadcast_5_v2}
& g_{n,s}^{k} \geq \sum_{\Jset \in \Hset | k \in Jset, n \notin \Jset} f_{n,\Jset}, \forall k \in \Nset, n \in \Nset - \{k\}
\end{align}
The device-centric stability region for the broadcast setup $\tilde{\Lambda}_d$ is defined as; $\tilde{\Lambda}_d = \{(A_{k}) |$ Eq.~(\ref{eq:appC_stab_reg_broadcast_5_v1}), Eq.~(\ref{eq:appC_stab_reg_broadcast_5_v2}), $g_{n,s}^{k} \geq 0, \forall n,k \in \Nset,  f_{n,\Jset} \geq \forall n \in \Nset, \Jset \in \Hset \}$. Next, we prove the stability statement in Theorem~\ref{eec_theorem1} for the broadcast setup.
%Eq.~(\ref{eq:appC_stab_reg_broadcast_4_v1}) and Eq.~(\ref{eq:appC_stab_reg_broadcast_4_v2}) define stability region of the device centric broadcast system. As it is seen, the device-centric stability region is smaller than the source-centric stability region by $\beta$ which could be arbitrarily small.

{\em Stability Proof:}
We consider the same Lyapunov function and drift considered for the unicast setup. Let us consider Eq.~(\ref{eq:appC_lyap_drift_4}) again. Since DcC sets ${g}_{k,n}^{k}(t) = \sum_{\Jset \in \Hset | k \in \Jset, n \notin \Jset} f_{n,\Jset}(t)$, $\forall k \in \Nset, n \in \Nset - \{k\}$ for broadcast scenario, Eq.~(\ref{eq:appC_lyap_drift_4}) is expressed as;
\begin{align} \label{eq:appC_lyap_drift_broadcast_1}
& \Delta(\boldsymbol H(t)) \leq B + 2E\biggl[ \sum_{k \in \Nset} {\lambda}_{k}(t) \Bigl( {y}_{k}(t) - {g}_{k,s}^{k}(t) - \nonumber \\
& \sum_{n \in \Nset - \{k\}} \sum_{\Jset \in \Hset | k \in \Jset, n \notin \Jset} {f}_{n, \Jset}(t)  \Bigr) + \sum_{k \in \Nset} \sum_{n \in \Nset - \{k\}}  \nonumber \\
& {\eta}_{n,k}(t) \Bigl(\sum_{\Jset \in \Hset | k \in \Jset, n \notin \Jset} {f}_{n, \Jset}(t) - {g}_{n,s}^{k}(t) \Bigr) +  \sum_{k \in \Nset}  \nonumber \\
& \sum_{n \in \Nset-\{k\}} Q_{n,k}(t) \Bigl( {x}_{n,k}(t) - {h}_{n,k}(t)  \Bigl) | \boldsymbol H(t)\biggr]
\end{align}
Considering that DcC sets ${x}_{n,k}(t) = {g}_{n,s}^{k}(t) - \beta$, $\forall k \in \Nset, n \in \Nset - \{k\}$, and ${h}_{n,k}(t) = {g}_{k,n}^{k}(t) = \sum_{\Jset \in \Hset | k \in \Jset, n \notin \Jset} f_{n,\Jset}(t)$, $\forall k \in \Nset, n \in \Nset - \{k\}$, the drift inequality in Eq.~(\ref{eq:appC_lyap_drift_broadcast_1}) is expressed as;
\begin{align} \label{eq:appC_lyap_drift_broadcast_2}
& \Delta(\boldsymbol H(t)) \leq B + 2E\biggl[ \sum_{k \in \Nset} {\lambda}_{k}(t) \Bigl( {y}_{k}(t) - {g}_{k,s}^{k}(t) - \nonumber \\
& \sum_{n \in \Nset - \{k\}} \sum_{\Jset \in \Hset | k \in \Jset, n \notin \Jset} {f}_{n, \Jset}(t)  \Bigr) + \sum_{k \in \Nset} \sum_{n \in \Nset - \{k\}}  \nonumber \\
& {\eta}_{n,k}(t) \Bigl(\sum_{\Jset \in \Hset | k \in \Jset, n \notin \Jset} {f}_{n, \Jset}(t) - {g}_{n,s}^{k}(t) \Bigr) +  \sum_{k \in \Nset}  \nonumber \\
 & \sum_{n \in \Nset-\{k\}} Q_{n,k}(t) \Bigl( {g}_{n,s}^{k}(t) - \beta - \sum_{\Jset \in \Hset | k \in \Jset, n \notin \Jset}  {f}_{n,\Jset}(t) \Bigl) \nonumber \\
&  | \boldsymbol H(t)\biggr]
\end{align}
Similar to the unicast setup, there exists a randomized policy with solution; $\oset{*}{g}_{k,s}^{k}(t)$, $\oset{*}{f}_{n,\Jset}(t)$, and satisfying;
\begin{align} \label{eq:appC_comp_w_randomized_ brodcast_1}
& - E \biggl[ \Bigl( \oset{*}{g}_{k,s}^{k}(t) + \sum_{n \in \Nset - \{k\}} \sum_{\Jset \in \Hset | k \in \Jset, n \notin \Jset} \oset{*}{f}_{n,\Jset}(t) -   \nonumber \\
& {y}_{k}(t)   \Bigr)  | \boldsymbol H(t) \biggr] \leq - \delta
\end{align}
\begin{align} \label{eq:appC_comp_w_randomized_brodcast_2}
& - E \biggl[\Bigl( \oset{*}{g}_{n,s}^{k}(t) - \sum_{\Jset \in \Hset | k \in \Jset, n \notin \Jset} \oset{*}{f}_{n,\Jset}(t)   \Bigr)  |  \boldsymbol H(t) \biggr] \leq  \nonumber \\
& -  \Bigl(  \beta - \delta \Bigr)
\end{align}
Since our algorithm, DcC, minimizes the right hand side of the drift inequality in Eq.~(\ref{eq:appC_lyap_drift_broadcast_2}), the solution of DcC, \ie ${g}_{k,s}^{k}(t)$, ${f}_{n,\Jset}(t)$, satisfy; $-$ $E [ {\lambda}_{k}(t)$ $( {g}_{k,s}^{k}(t)$ $+$ $\sum_{n \in \Nset - \{k\}}$ $\sum_{\Jset \in \Hset | k \in \Jset, n \notin \Jset}$ ${f}_{n,\Jset}(t)$ $-$  ${y}_{k}(t)   )$ $|$ $\boldsymbol H(t) ]$ $\leq$ $-$ $E [ {\lambda}_{k}(t)$ $( \oset{*}{g}_{k,s}^{k}(t)$ $+$ $\sum_{n \in \Nset - \{k\}}$ $\sum_{\Jset \in \Hset | k \in \Jset, n \notin \Jset}$ $\oset{*}{f}_{n,\Jset}(t)$ $-$  ${y}_{k}(t)   )$ $ |$ $\boldsymbol H(t) ]$ $\leq$ $-$ ${\lambda}_{k}(t)$ $\delta $ and $-$ $E [ ( {\eta}_{n,k}(t)$ $-$ $Q_{n,k}(t) )$ $( {g}_{n,s}^{k}(t)$ $-$ $\sum_{\Jset \in \Hset | k \in \Jset, n \notin \Jset}$ ${f}_{n,\Jset}(t)   )$  $|$  $\boldsymbol H(t) ]$ $\leq$ $-$ $E [ ( {\eta}_{n,k}(t)$ $-$ $Q_{n,k}(t) )$ $( \oset{*}{g}_{n,s}^{k}(t)$ $-$ $\sum_{\Jset \in \Hset | k \in \Jset, n \notin \Jset}$ $\oset{*}{f}_{n,\Jset}(t)   )$  $|$  $\boldsymbol H(t) ]$ $\leq$  $-$ $( {\eta}_{n,k}(t)$ $-$ $Q_{n,k}(t) )$ $(  \beta$ $-$ $\delta )$. By taking into account these inequalities, the drift inequality in Eq.~(\ref{eq:appC_lyap_drift_broadcast_2}) is bounded as;
\begin{align} \label{eq:appC_lyap_drift_broadcast_3}
& \Delta(\boldsymbol H(t)) \leq B - 2E\biggl[ \sum_{k \in \Nset} {\lambda}_{k}(t) \delta + \sum_{k \in \Nset} \sum_{n \in \Nset - \{k\}}   \nonumber \\
& {\eta}_{n,k}(t) \Bigl( \beta - \delta \Bigr) +  \sum_{k \in \Nset} \sum_{n \in \Nset-\{k\}} Q_{n,k}(t) \delta | \boldsymbol H(t)\biggr]
\end{align} Since $\beta > \delta$, the time average of the Lyapunov drift in Eq.~(\ref{eq:appC_lyap_drift_broadcast_3}) shows that the time average of the sum of the queues are bounded. This concludes the proof for the broadcast setup.
