# Supplementary material for: Device-Aware Routing and Scheduling in Multi-Hop Device-to-Device Networks
Source: arXiv:1708.06475 source file (2017-08-22)
Supplement: Supplementary file 3 [file appendixC.tex]

%\vspace{-5pt}
\section*{Appendix C: Proof of Theorem~\ref{eec_theorem2}}
%\vspace{-5pt}
Let us consider the proof of Theorem~\ref{eec_theorem2} for the unicast setup. The proof for the broadcast setup directly follows from Appendix A.B and Appendix A.C.

Let define a drift-plus-penalty function as $\Delta(\boldsymbol H(t)) - \sum_{k \in \Nset} M E[ U_{k}({y}_{k}(t)) | \boldsymbol H(t)]$ which is, considering the bounds presented in Appendix A.A, bounded as;
\begin{align} \label{eq:appC_opt_1}
& \Delta(\boldsymbol H(t)) - \sum_{k \in \Nset} M E\biggl[ U_{k}({y}_{k}(t)) | \boldsymbol H(t) \biggr] \leq B -  2E\biggl[   \nonumber \\
& \sum_{k \in \Nset} {\lambda}_{k}(t) \Bigl( {g}_{k,s}^{k}(t) + \sum_{n \in \Nset - \{k\}} {g}_{k,n}^{k}(t)  - {y}_{k}(t) \Bigr)  + \sum_{k \in \Nset}  \nonumber \\
& \sum_{n \in \Nset - \{k\}} \Bigl( {\eta}_{n,k}(t) - Q_{n,k}(t) \Bigr) \Bigl( {g}_{n,s}^{k}(t) -  {g}_{k,n}^{k}(t) \Bigr)  +  \nonumber \\
& \sum_{k \in \Nset} \sum_{n \in \Nset-\{k\}} Q_{n,k}(t) \beta | \boldsymbol H(t)\biggr]  - \sum_{k \in \Nset} M E\biggl[ U_{k}({y}_{k}(t)) \nonumber \\
& | \boldsymbol H(t) \biggr]
\end{align} Note that the minimization of the right hand side of the drift inequality in Eq.~(\ref{eq:appC_opt_1}) corresponds to the cellular link scheduler in Eq.~(\ref{eq:cellular_scheduling}) and the local area link scheduler for unicast in Eq.~(\ref{eq:local_area_scheduling_unicast}), and the rate control in Eq.~(\ref{eq:rate_control}). Also, note that the existence of finite positive constant $B$ in Eq.~(\ref{eq:appC_opt_1}) depends on positive finite value of $R_{k}^{max}$ in Eq.~(\ref{eq:rate_control}) \cite{neelybook}.

Since there exists a randomized algorithm satisfying $-$ $E [$ $\lambda_{k}(t)$ $( {g}_{k,s}^{k}(t)$ $+$ $\sum_{n \in \Nset - \{k\}}$ ${g}_{k,n}^{k}(t)$ $-$ ${y}_{k}(t)  )$ $|$ $\boldsymbol H(t) ]$ $\leq$ $-$ $E [ \lambda_{k}(t)$ $( \oset{*}{g}_{k,s}^{k}(t)$ $+$ $\sum_{n \in \Nset - \{k\}}$ $\oset{*}{g}_{k,n}^{k}(t)$ $-$ ${y}_{k}(t)   )$ $|$ $\boldsymbol H(t) ]$ $\leq$  $-$ ${\lambda}_{k}(t)$ $\delta $ and $-$ $E [$ $( {\eta}_{n,k}(t)$ $-$ $Q_{n,k}(t) )$ $({g}_{n,s}^{k}(t)$ $-$ ${g}_{k,n}^{k}(t)   )$ $|$ $\boldsymbol H(t) ]$ $\leq$ $-$ $E [ ( {\eta}_{n,k}(t)$ $-$ $Q_{n,k}(t) )$ $( \oset{*}{g}_{n,s}^{k}(t)$ $-$ $\oset{*}{g}_{k,n}^{k}(t)   )$ $|$ $\boldsymbol H(t) ]$ $\leq$  $-$ $( {\eta}_{n,k}(t)$ $-$ $Q_{n,k}(t) )$ $(  \beta$ $-$ $\delta )$, the right hand side of Eq.~(\ref{eq:appC_opt_1}) is bounded as;

\begin{align} \label{eq:appC_opt_2}
& \Delta(\boldsymbol H(t)) - \sum_{k \in \Nset} M  E\biggl[ U_{k}({y}_{k}(t)) | \boldsymbol H(t) \biggr]  \leq B - 2 \sum_{k \in \Nset} \nonumber \\
&  {\lambda}_{k}(t) \delta  - 2 \sum_{k \in \Nset} \sum_{n \in \Nset - \{k\}} {\eta}_{n,k}(t) (\beta - \delta) -  2 \sum_{k \in \Nset}   \nonumber \\
& \sum_{n \in \Nset - \{k\}} Q_{n,k}(t) \delta - \sum_{k \in \Nset} M E[U_{k}(A_{k}+\delta)]
\end{align}
where $\sum_{k \in \Nset} U_{k}(A_{k})$ is the maximum time average of the sum utility function that can be achieved by any control policy that stabilizes the system. Let $\epsilon = \max\{\delta, \beta-\delta\}$. Then, the time average of Eq.~(\ref{eq:appC_opt_2}) becomes;
\begin{align} 
& \limsup_{t \rightarrow \infty} \frac{1}{t} \sum_{\tau = 0}^{t-1} \biggl[\Delta(\boldsymbol H(\tau))  - \sum_{k \in \Nset} M E[U_{k}(y_{k}(\tau))] \biggr] \leq \nonumber \\
&  \limsup_{t \rightarrow \infty}  \frac{1}{t} \sum_{\tau = 0}^{t-1} \biggl[ B - 2 \sum_{k \in \Nset} \lambda_{k} (\tau) \epsilon - 2 \sum_{k \in \Nset} \sum_{n \in \Nset - \{k\}}  \nonumber
\end{align}
\begin{align} \label{eq:appC_opt_4}
& \eta_{n,k}(\tau) \epsilon - 2 \sum_{k \in \Nset} \sum_{n \in \Nset - \{k\}} Q_{n,k}(\tau) \epsilon - \sum_{k \in  \Nset} M U_{k}(A_{k} \nonumber \\
& +\epsilon) \biggr]
\end{align}

Let us first consider the stability of the queues. If both sides of Eq.~(\ref{eq:appC_opt_4}) are divided by $\epsilon$ and the terms are arranged, we have;
\begin{align} \label{eq:appC_opt_5}
& \limsup_{t \rightarrow \infty} \frac{1}{t} \sum_{\tau = 0}^{t-1} \biggl[ \sum_{k \in \Nset} \lambda_{k}(\tau) + \sum_{k \in \Nset} \sum_{n \in \Nset - \{k\}} \eta_{n,k} (\tau) \nonumber \\
& + \sum_{k \in \Nset} \sum_{n \in \Nset - \{k\}} Q_{n,k}(\tau) \biggr]  \leq \frac{B}{2\epsilon}  + \limsup_{t \rightarrow \infty} \frac{1}{t} \sum_{\tau = 0}^{t-1} \biggl[ \sum_{k \in \Nset}  \nonumber \\
& \frac{M}{\epsilon} E[U_{k}(y_{k}(\tau))]  \biggr] - \sum_{k \in \Nset} \frac{MU_{k}(A_{k}+\epsilon)}{\epsilon}
\end{align} which concludes that the time average of the queue sizes are bounded, so DcC stabilizes the queues in the system.

Now, let us consider the optimality. If both sides of Eq.~(\ref{eq:appC_opt_4}) are divided by $M$, we have;
\begin{align} \label{eq:appC_opt_6}
& \limsup_{t \rightarrow \infty} \frac{1}{t} \sum_{\tau = 0}^{t-1} \biggl[ - \sum_{k \in \Nset} E[U_{k} (y_{k} (\tau)) ] \biggr] \leq
\limsup_{t \rightarrow \infty} \frac{1}{t} \sum_{\tau = 0}^{t-1} \biggl[ \nonumber \\
& \frac{B}{M}  - 2 \sum_{k \in \Nset} \lambda_{k}(\tau) \frac{\epsilon}{M}  - 2 \sum_{k \in \Nset} \sum_{k \in \Nset - \{k\}} \eta_{n,k}(\tau) \frac{\epsilon}{M} -  \nonumber \\
& 2 \sum_{k \in \Nset} \sum_{n \in \Nset - \{k\}} Q_{n,k}(\tau)\frac{\epsilon}{M} - \sum_{k \in \Nset} U_{k} (A_{k} + \epsilon)  \biggr]
\end{align} By arranging the terms we have;
\begin{align} \label{eq:appC_opt_7}
& \limsup_{t \rightarrow \infty} \frac{1}{t} \sum_{\tau = 0}^{t-1} \biggl[ \sum_{k \in \Nset} E[U_{k} (y_{k} (\tau)) ] \biggr] \geq
\limsup_{t \rightarrow \infty} \frac{1}{t} \sum_{\tau = 0}^{t-1} \biggl[  \nonumber \\
& \sum_{k \in \Nset} U_{k}(A_{k}+\epsilon) - \frac{B}{M} + 2 \sum_{k \in \Nset} \lambda_{k}(\tau)\frac{\epsilon}{M} + 2 \sum_{k \in \Nset} \nonumber \\
& \sum_{n \in \Nset - \{k\}}  \eta_{n,k}(\tau)  \frac{\epsilon}{M} + 2 \sum_{k \in \Nset} \sum_{n \in \Nset - \{k\}} Q_{n,k}(\tau) \frac{\epsilon}{M} \biggr]
\end{align} The following inequality is straightforward from Eq.~(\ref{eq:appC_opt_7}).
%\begin{align} \label{eq:appC_opt_8}
%& \limsup_{t \rightarrow \infty} \frac{1}{t} \sum_{\tau = 0}^{t-1} \biggl[ \sum_{k \in \Nset} E[U_{k} (y_{k} (\tau)) ] \biggr] \geq
%\limsup_{t \rightarrow \infty} \frac{1}{t} \sum_{\tau = 0}^{t-1} \biggl[  \nonumber \\
%& \sum_{k \in \Nset} U_{k}(A_{k}+\epsilon) - \frac{B}{M} \biggr]
%\end{align} which leads to
\begin{align} \label{eq:appC_opt_9}
& \limsup_{t \rightarrow \infty} \frac{1}{t} \sum_{\tau = 0}^{t-1} \biggl[ \sum_{k \in \Nset} E[U_{k} (y_{k} (\tau)) ] \biggr] \geq
 \sum_{k \in \Nset}  U_{k}(A_{k}+\epsilon) \nonumber \\
&  - \frac{B}{M}
\end{align} This proves that the admitted flow rate by DcC converge to the utility optimal operating point with increasing $M$. This concludes the proof.
